# Supplementary material for: First principle prediction of structural distortions in the cuprates and their impact on the electronic structure
Source: arXiv:2309.07997 source file (2024-11-01)
Supplement: Supplementary file 1 [file supp.pdf]

# Supplementary materials for "First principle prediction of structural distortions in the cuprates and their impact on the electronic structure"

Zheting Jin[1] and Sohrab Ismail-Beigi[1,2,3]

[1]*Department of Applied Physics, Yale University, New Haven, Connecticut 06520, USA*

[2]*Department of Physics, Yale University, New Haven, Connecticut 06520, USA*

[3]*Department of Mechanical Engineering and Materials Science, Yale University, New Haven, CT 06520, USA*

(Dated: October 23, 2024)

**Contents**

**I. Convergence of the calculations** 3

A. Undoped system 3

B. Hole-doped system 5

**II. Stable or meta-stable crystals and their energies** 6

A. Undoped system 6

B. Hole-doped system 8

**III. Necessity of $U$ functional** 8

**IV. Functional comparisons** 10

A. Undoped system 10

B. Hole doped system 14

**V. Wannierization** 15

**VI. Uniform magnetic states and their energies in hole-doped system** 20

**VII. DFT orbitals vs Wannier orbitals** 20

**VIII. Summary of computational details** 23

A. SIESTA 23

B. VASP 23

**References** 23

# I. CONVERGENCE OF THE CALCULATIONS

All the crystal and electronic structure calculations presented in this work use the 5.4.4 version of the VASP software [1, 2], which is a plane-wave-based DFT code. In VASP, two parameters heavily influence the computational convergence: the plane-wave energy cutoff (ENCUT parameter), which controls the completeness of the basis set, and the $k$-mesh density used for sampling the Brillouin zone (KPOINTS file). To ensure the accuracy of calculations, it is essential to determine the minimum required values of these parameters through testing before conducting production runs, as these values can vary depending on specific systems.

To avoid too much computational effort, we only aim to converge the energy difference of various crystal or spin structures up to 1meV per Cu atom. All the VASP calculations come with an energy tolerance of EDIFF $= 10^{-5}$eV and a force tolerance of EDIFFG $= -3 \times 10^{-2}$eV/Å. Gaussian smearing of 0.2eV is used for SCF calculations, which is the largest smearing with a small enough entropy effect $E - F < 1$meV/Cu.

## A. Undoped system

We start the tests with the undoped system. For undoped Bi-2212, we studied a 60-atom bulk unit cell, with 2 Cu atoms per CuO layer. The lattice constants are about 5.43Å, 5.49Å, and 31.98Å. We focus our convergence tests on two representative fixed crystal structures: the high-symmetry crystal in Fig.1(b) of the main article and the low-symmetry chain crystal in Fig.2(b) of the main article. In this supplementary material, Fig.S 1(a) shows the total energies of these two crystals as a function of the plane-wave cutoff energy $E_c$. Both crystals start to converge when $E_c > 500$eV. In addition, the total energy difference between the two crystals is more important in this work. Fig.S 1(b) shows the energy difference per Cu atom as a function of $E_c$. The energy difference starts to converge to a precision of 1meV/Cu when $E_c > 400$eV. To ensure convergence, we allow some redundancy and use a relatively high plane-wave cutoff energy of 500eV in our main results.

Fig.S 1(c-d) shows the total energy and energy difference per Cu atom as functions of $k$-spacing along $c$-direction. One $k$-point along $c$-direction turns out to be enough to precisely converge the energy difference. This is because of the long lattice constant along $c$-axis (31.98Å). Fig.S 1(e) shows the total energy as a function of $k$-spacing along $b$-direction, where we fix the $k$-mesh along $c$-axis to be one, and have the same $k$-mesh along $a$- and $b$-axis. Hence the $k$-spacing along $a$-

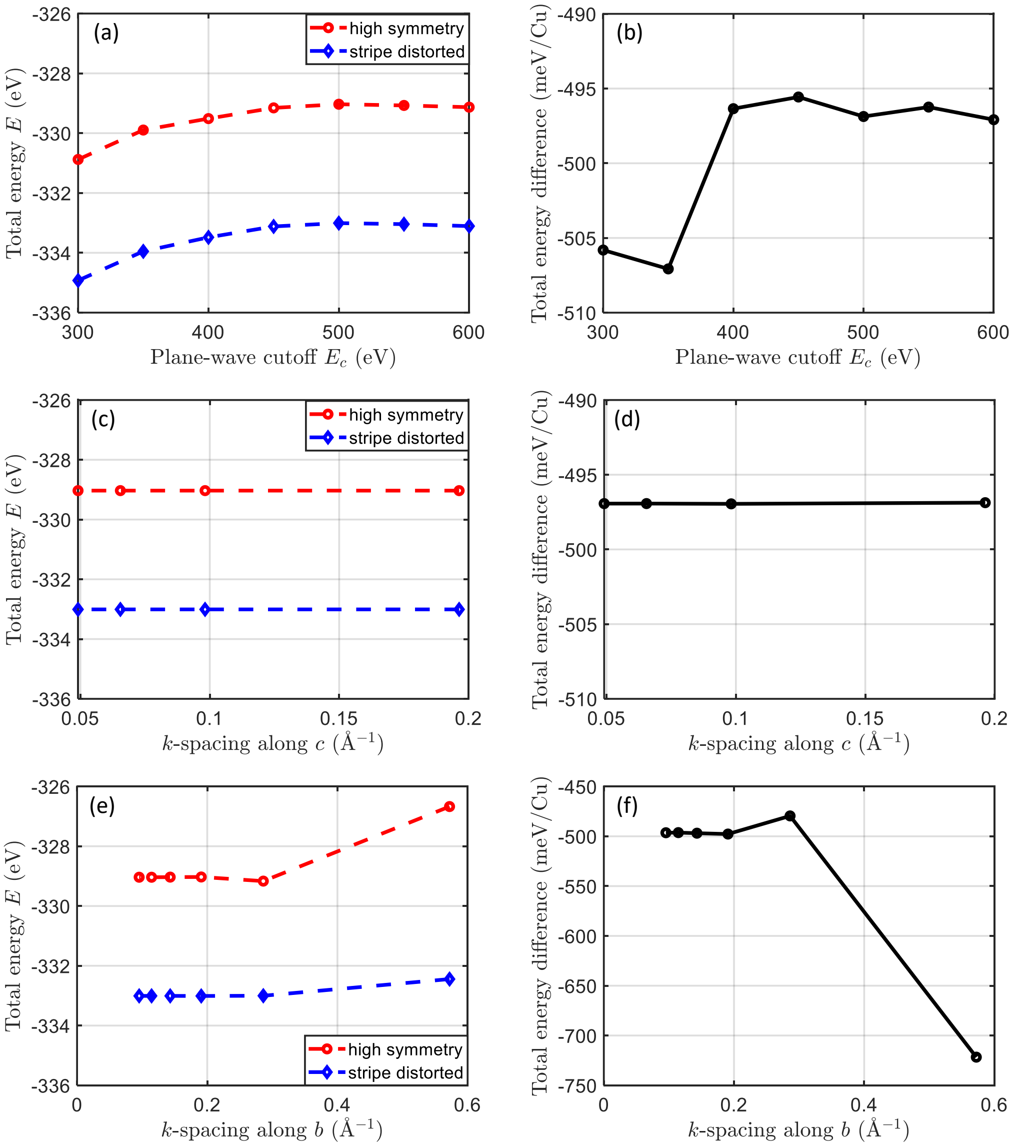


Fig.S 1: The convergence of total energy and the energy difference versus plane-wave cutoff energy and the $k$-mesh density of the undoped Bi-2212. (a) Total energy $E$ as a function of the plan-wave cutoff energy $E_c$ in VASP. Red circles and blue diamonds represent the results of the high-symmetry and chain-distorted crystals, respectively. (b) The total energy difference between the two crystals in (a): $E_{chain} - E_{highsym}$ divided by the number of Cu atoms shows the energy difference per Cu atom. (c) Total energy $E$ as a function of $k$-spacing along $c$ direction. The data points from left to right come from $k$-mesh of $8 \times 8 \times 1$, $8 \times 8 \times 2$, $8 \times 8 \times 3$, and $8 \times 8 \times 4$, respectively. (d) The total energy difference per Cu atom between the two crystals as a function of $k$-spacing along $c$ direction. The $k$-spacing describes the distance between two nearest $k$ points defined as $2\pi/(cN_c)$, where $c$ is the lattice constant and $N_c$ is the number of $k$ grids along the corresponding direction. (e-f) The total energy or energy per Cu as a function of $k$-spacing along $b$ direction. The data points from left to right come from $k$-mesh of $12 \times 12 \times 1$, $10 \times 10 \times 1$, $8 \times 8 \times 1$, $6 \times 6 \times 1$, $4 \times 4 \times 1$, and $2 \times 2 \times 1$, respectively.

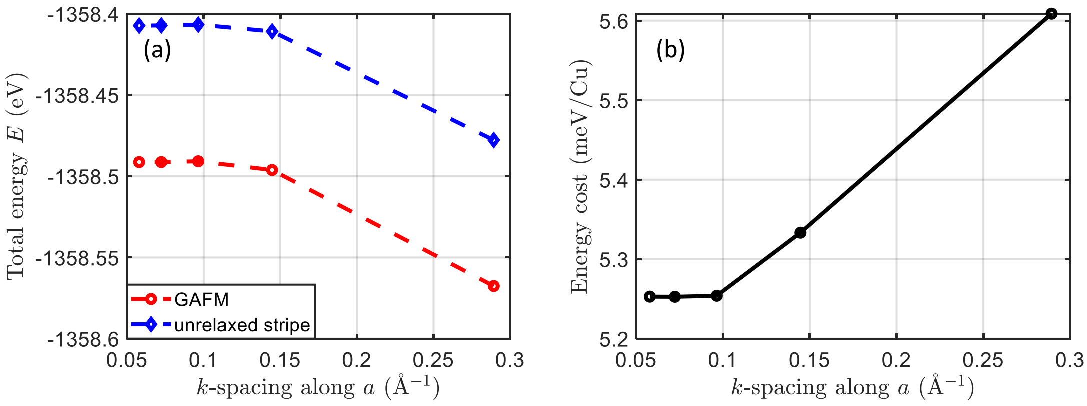


Fig.S 2: The convergence of total energy and the energy difference versus the $k$-mesh density of the hole-doped Bi-2212. (a) Total energy $E$ as a function of $k$-spacing along $a$ direction. Red circles and blue diamonds represent the results of the GAFM state and a representative stripe order state using the same fixed crystal structure. All data points use a dense enough $k$-mesh of 8 and 1 along $b$ and $c$ directions according to the results in Fig.S 1. As for the $a$-axis, data points from left to right come from $k$-mesh of 5, 4, 3, 2, and 1, respectively. (b) The energy difference between the stripe order state and G-AFM state: $E_{\text{stripe}} - E_{\text{GAFM}}$ divided by the number of Cu atoms.

direction is almost the same as the one along $b$-axis due to similar lattice constants on these two axes. Both Fig.S 1(e) and (f) show convergence at the $6 \times 6 \times 1$ $k$-mesh, and we again use a relatively denser $k$-mesh of $8 \times 8 \times 1$ in our main results.

While the $8 \times 8 \times 1$ $k$-mesh with Gaussian smearing of 0.2eV converges the energy differences, the convergence of the density of states requires a much denser $k$-mesh. The density of states provided in the main article comes from a denser $k$-mesh of $30 \times 30 \times 3$ with a smaller smearing of 0.04eV.

## B. Hole-doped system

For the hole-doped system, we considered a 244-atom unit cell, which starts from a $4 \times 1 \times 1$ bulk supercell of the undoped system. Then 25% hole doping is introduced by 4 interstitial oxygen dopants in the crystal. The most energetically favorable crystal structure is the one shown in Fig.3 of the main article, and we will also provide a set of meta-stable crystals and the corresponding energies in Supp. Sec. II B.

The $4 \times 1 \times 1$ larger unit cell in the hole-doped system requires less $k$-mesh along $a$-axis to reach

the converged $k$-spacing in the undoped system. Fig.S 2 shows a convergence test of the $k$-spacing along $a$-axis, where we are converging the total energy and the energy difference between the stripe order state and G-AFM state. We find that the $2 \times 8 \times 1$ $k$-mesh is enough to converge the total energy and the energy different to 1meV/Cu, but we again allow some redundancy and use $3 \times 8 \times 1$ $k$-mesh in our main results.

## II. STABLE OR META-STABLE CRYSTALS AND THEIR ENERGIES

During the crystal structural relaxation calculations, we found a lot of meta-stable crystals in addition to the most energetically favorable crystals. In this section, we will show some typical meta-stable crystals and the corresponding total energies of these crystals.

### A. Undoped system

The meta-stable crystals in the undoped systems have several typical Bi-O distortion patterns as shown in Fig.S 3(b-d). Compared to the high-symmetry crystal structure in Fig.S 3(a), these crystals have shorter Bi-O bond lengths and lower total energies. In principle, all four crystals should have the 2 Cu/layer unit cells marked by the black squares due to the GAFM order in the Cu-O plane. However, the high-symmetry and zig-zag crystals in Fig.S 3(a)(c) show a smaller translational repeating cell on the Bi-O layer, marked by the blue dashed squares, which is a 1Cu/layer cell. Using this small cell, the zig-zag crystal has been discovered in previous work [3], but the in-plane AFM order is artificially removed due to the choice of the small 1Cu/layer unit cell. Fig.S 3(b) shows a diamond-shape distortion pattern, whose energy is relatively close to the lowest-energy crystal with the orthorhombic distortion pattern in Fig.S 3(d). As we will show in the hole-doped system part in Supp. Sec. II B, the diamond and orthorhombic distortion patterns co-exist when we introduce additional oxygen dopants into the system.

Furthermore, we find that the lower energy crystals always come with shorter Bi-O bond lengths. Fig. 3(e) show the energy per Cu atom as a function of Bi-O bond length, where the high-symmetry crystal is chosen to be an energy reference. As an example, the chain pattern shows the shortest Bi-O bond length as well as the lowest total energy. This is because shorter bond lengths come with larger Bi-O couplings, which lower the energy of the Bi-O bonding state and raise the energy of the antibonding state. Since the Bi-O antibonding state is almost empty, the total energy is dominated by the energy of the occupied bonding state, which is lower in the crystal with shorter

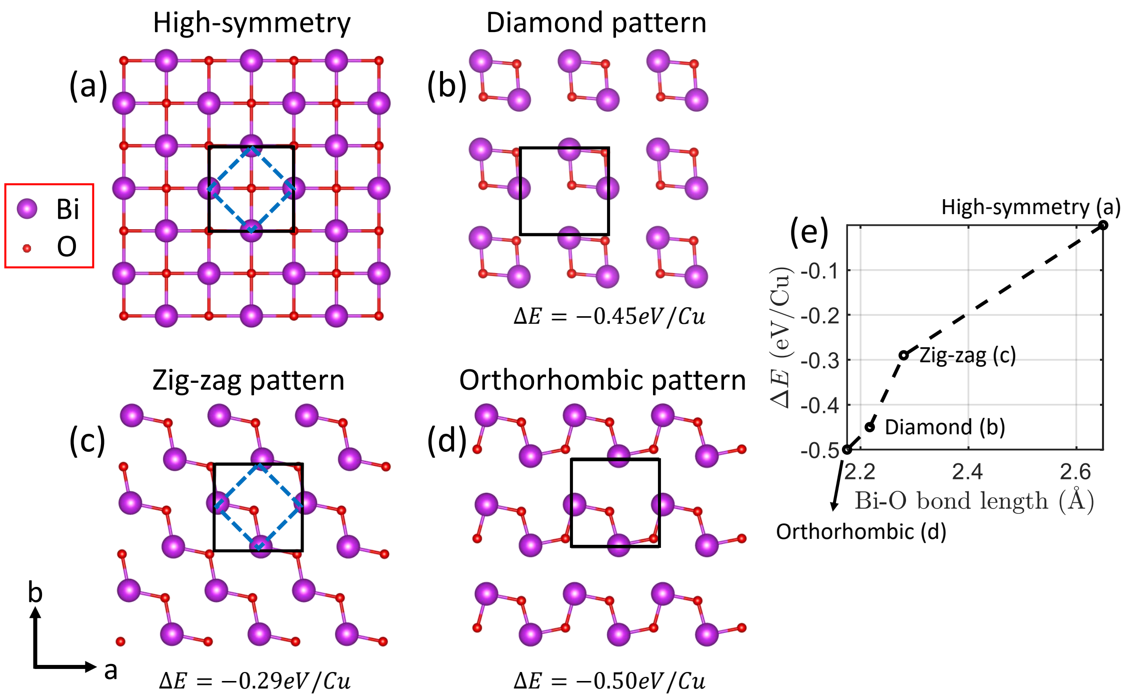


Fig.S 3: Typical distortion patterns of the Bi-O layer and their effects on the total energies. Here we show the top view of the Bi-O layer, where the magenta large balls are Bi and the red small balls are O atoms. The black squares represent the unit cells. (a) The high-symmetry crystal (tetragonal). (b) Diamond-shaped distortion pattern (tetragonal). (c) Zig-zag distortion pattern (tetragonal). (d) Orthorhombic distortion pattern. Compared to the high-symmetry crystal in (a), the low-symmetry structures in (b-d) are more energetically favorable by $\Delta E$. (e) $\Delta E$ as a function of Bi-O bond length in each crystal.

Bi-O bonds. This mechanism is also crucial to the insulating property as discussed in the main article.

From the above analysis, the distortion pattern of the Bi-O layer greatly affects the total energy, by about 0.3 to 0.5eV per Cu atom compared to the high-symmetry crystal. In addition, inter-layer coupling also slightly affects the total energy. Focusing on the orthorhombic distortion pattern, we find that the two Bi-O layers in the same bilayer should show the same top view to achieve the lowest energy crystal. This observation is consistent with previous work [4]. Other different orientations between the two layers can influence the total energy by about 25meV/Cu, one order of magnitude smaller than the effect of Bi-O distortions. The inter-bilayer coupling, however, makes very little difference to the total energy, less than 3meV/Cu. This is the reason why many previous works chose to only study one bilayer and completely ignore the inter-bilayer couplings [4–7].

### B. Hole-doped system

The hole-doped system starts from a 4×1×1 repeat of the undoped system with 4 interstitial oxygen dopants, adding up to 244 atoms in the unit cell. There are in principle too many possible configurations of oxygen dopant positions to study in this huge unit cell, so here we only list several typical meta-stable structures as an example. Note that several previous works [4, 5] have also studied the realistic oxygen dopant positions in the bilayer slabs, and they used smaller unit cells. The interstitial oxygen dopants between Sr and Bi layers show the lowest energy, several electron volts lower than other meta-stable positions [5]. Such a huge difference in energy will not be inverted even if we study large unit cells and bulks. For that reason, the most energetically favorable positions of the oxygen dopants should still be either between Sr and Bi layers as shown in the previous works, or between two Bi layers, which is missing in previous slab studies.

Fig.S 4(a) shows the lowest energy crystal used in the main article. As a comparison, we list several typical meta-stable crystals and list the corresponding energy difference compared to the lowest energy crystal. In Fig.S 4(b), the pair of oxygen dopants marked by the red arrows are aligned along $c$-direction instead of the diagonal direction shown in panel (a). This change cost $\Delta E = 168$meV compared to the lowest energy crystal. In Fig.S 4(c), all pairs of oxygen dopants are aligned in parallel. This crystal shows 183meV higher energy compared to the staggered aligned oxygen dopants in panel (a). The crystal in Fig.S 4(d) is very similar to the lowest energy structure, except for a different local distortion pattern at the oxygen dopant marked by the red arrow. The distortion pattern is centered at a nearby Bi atom instead of centered at the oxygen dopant as shown at all other oxygen dopants. Fig.S 4(e-f) show two kinds of meta-stable structures where oxygen dopants locate between two Bi layers and the dopants are either close to or far from each other. These two structures have much higher energy, one order of magnitude larger than the energy cost of moving oxygen dopants between Sr and Bi layers as shown in Fig.S 4(b-d).

## III. NECESSITY OF $U$ FUNCTIONAL

The DFT calculations have some well-known limitations [8]. For example, the local-density approximation (LDA) tends to underestimate the band gap, especially in semiconductors and insulators, by approximately 40% [9]. This limitation is attributed to self-interaction errors (SIE) in the approximate exchange-correlation functionals [10]. As an improvement, DFT+U [11] applies the Hubbard $U$ correction exclusively to a specific subset of states in the system, usually of $d$- or

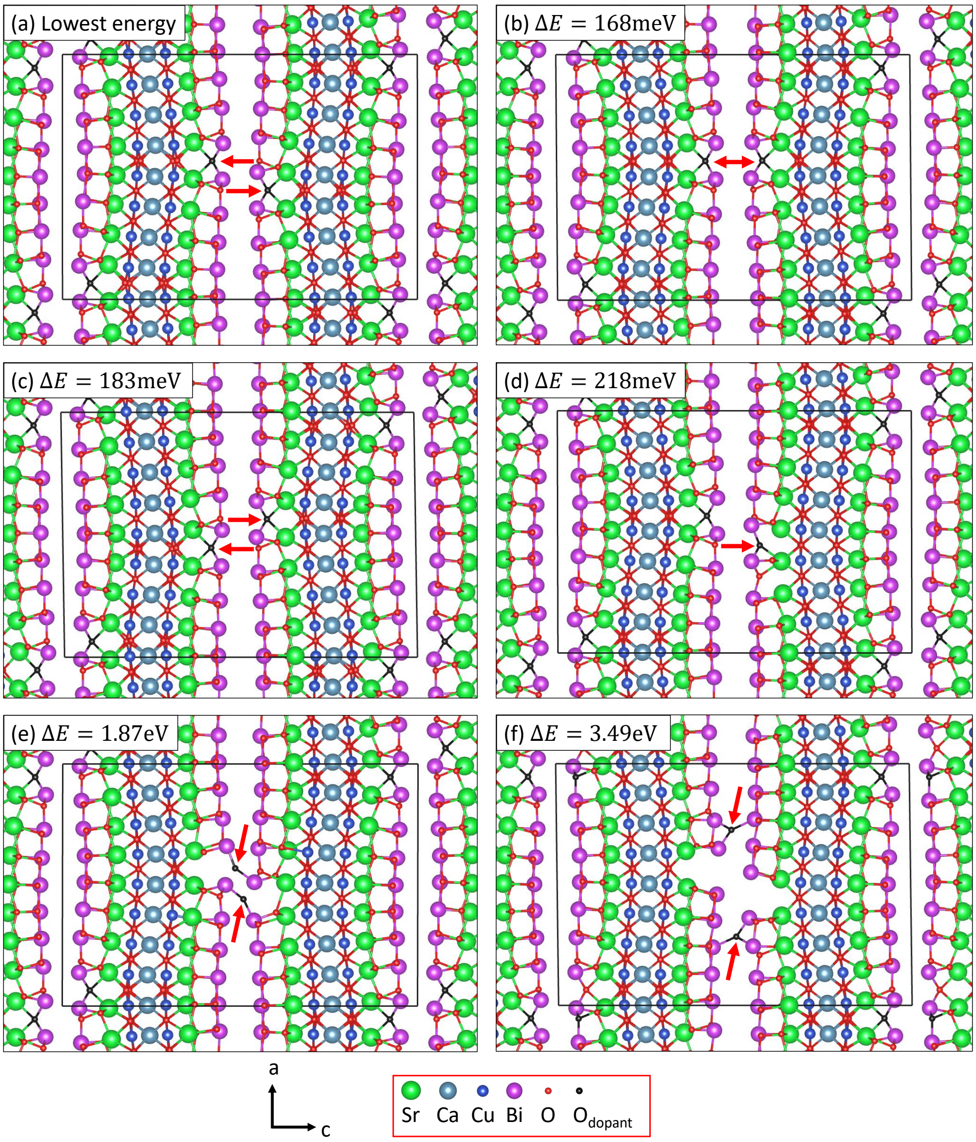


Fig.S 4: Typical meta-stable crystals of the hole-doped systems and the corresponding total energies compared to the lowest energy crystal. Black balls represent the oxygen dopants. (a) The lowest energy crystal. (b-f) are crystals similar to (a), except for some small differences in the following: (b) One pair of the oxygen dopants are aligned along $c$-direction as marked by the red arrows. (c) All pairs of oxygen dopants are aligned in parallel. (d) The oxygen dopant marked by the red arrow introduces a Bi-O distortion centered at a nearby Bi atom. (e-f) The oxygen dopants are between two Bi-O layers.

$f$-shells. This approach greatly improves the band gap predicted by DFT, especially in transition metal oxides [12]. Within the GGA+$U$ framework, the optimal $U$ for copper oxides to reproduce experimental magnetic moment and band gap is 4eV [13]. This $U$ value has also been used in prior

theoretical works in BSCCO [3, 14].

In the meantime, several meta-GGA functionals have been developed to improve the prediction of band gaps in DFT, such as the strongly constrained and appropriately normed semilocal density functional (SCAN) [15]. However, SCAN functional still displays shortcomings such as overestimating local magnetic moments in magnetic systems [16, 17], underestimating band gaps [18], and failure to reproduce insulating ground state in CuO. A more recent SCAN+U method makes use of the DFT+$U$ approach to improve the SCAN functional, where the optimal $U$ for copper oxides to reproduce experimental magnetic moment and band gap is 2eV [19].

Therefore, to avoid the known failure of the LDA, GGA, and SCAN in reproducing the insulating ground state in undoped BSCCO [5–7, 20–24], we add the $U$ functional to reduce the self-interaction errors.

## IV. FUNCTIONAL COMPARISONS

An inevitable discussion about DFT studies is the choice of the DFT functional. In the main article, we follow prior theoretical works [3, 13, 14] and use PBE+$U$ functional with $U = 4$ eV. There are in principle several more advanced functional with heavier computational costs, such as SCAN+$U$ functional [18, 19]. For cuprates, while $U = 4$ eV [3, 13, 14] is usually used in PBE+$U$ functional, the SCAN+$U$ functional usually requires $U = 2$ eV for the Cu-d orbitals. For example, while the SCAN functional fails to predict any finite insulator gap for CuO, SCAN+$U$ with $U = 2$ eV reproduces the experimental insulator band gap and local moment [19].

In this section, we compare the PBE+$U$ and SCAN+$U$ functional in BSCCO, by exploring the ground state band structures with different $U$ values. In particular, the results from PBE+$U$ with $U = 4$ eV and SCAN+$U$ with $U = 2$ eV only show a negligible difference, so we choose to convey our main study using the computationally easier PBE+$U$ functional. In addition, our results are qualitatively insensitive to the value of $U$ when it is larger than 2eV in both PBE+$U$ and SCAN+$U$ calculations.

### A. Undoped system

We start the tests with the undoped system. For undoped Bi-2212, we studied a 60-atom bulk unit cell, with 2 Cu atoms per CuO layer. The crystal structure used in all calculations in this subsection is the orthorhombic distorted undoped crystal as shown in Fig.S 3(d). In all

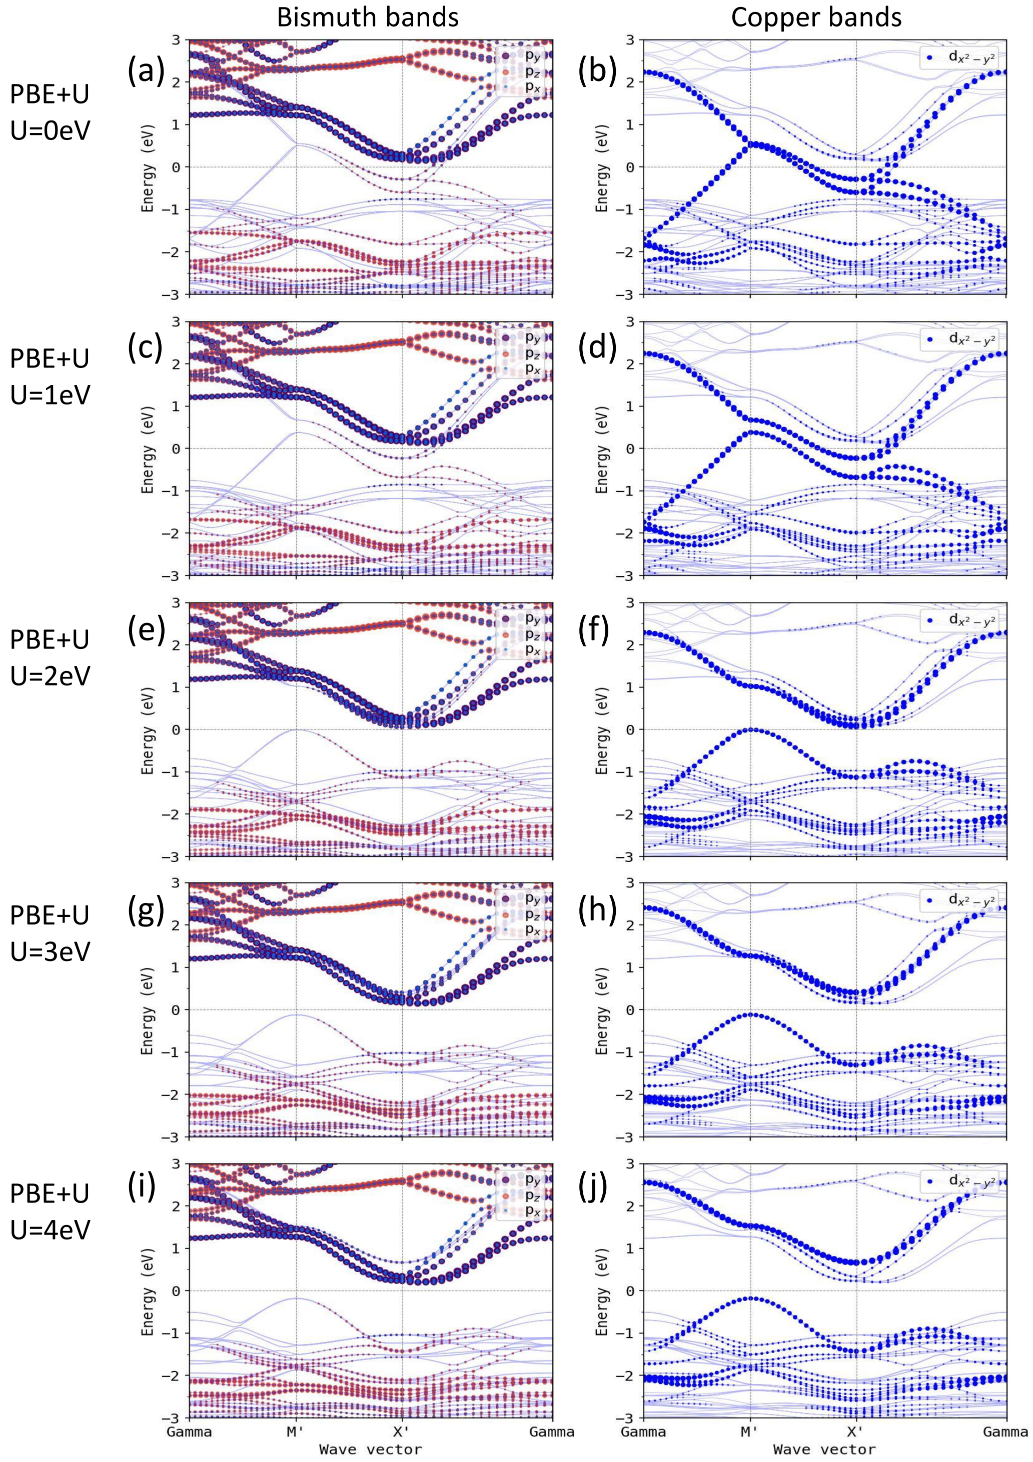


Fig.S 5: Projected band structures on the Bi $p$-orbitals and Cu $d_{x^2-y^2}$ orbitals from PBE+$U$, with different $U$ values. Panels (a-b), (c-d), (e-f), (g-h), and (i-j) are the results of PBE+$U$ with $U$ =0, 1, 2, 3, and 4eV, respectively. Panels (a)(c)(e)(g)(i) show the projections on Bi $p$-orbitals while panels (b)(d)(f)(h)(j) show Cu $d_{x^2-y^2}$ orbitals.

calculations, we fully relax the bulk crystals and then study the electronic structures. Using the PBE functional, or equivalent PBE+$U$ functional with $U = 0$, we reproduce the non-magnetic metallic ground states predicted by prior works using LDA/GGA functionals [6, 7, 20–24]. Note that regardless of the U values, the bismuth bands in Fig.S 5(a), (c), (e), (g), and (i) are always insulating. This discovery is consistent with experiments, where there has never been a bismuth electron pocket seen in BSCCO, despite the doping levels. The physical origin of the insulating Bi bands in the chain pattern is discussed in the "Undoped system" section in the main article and the Wannierization study in Supp. Sec. V.

As we increase the $U$ values in PBE+$U$ calculations, the undoped system gradually develops AFM order and opens a corresponding AFM gap for the Cu bands. The $U$ = 1eV calculation in Fig.S 5(c-d) still shows a metallic ground state with a relatively small local moment of about 0.13$\mu_B$, much smaller than the experimental measurements on local moments of about 0.4-0.6$\mu_B$ [25, 26] in cuprates without chlorine. The $U$ = 2eV calculation in Fig.S 5(e-f) comes with a local moment of 0.41$\mu_B$ and a large enough AFM ordering gap, which raises high-energy Cu $d_{x^2-y^2}$ band above the antibonding BiO band, resulting in an AFM insulating ground state. Note that $U$ = 2eV is also the lowest required $U$ to open an indirect band gap for the Cu-$d_{x^2-y^2}$ bands in Fig.S 5(f). We use $U$ = 4eV in our main article because it is a common choice for copper $d$-orbitals in Bi-2212 [3, 14], and the same $U$ value has quantitatively reproduced a wide range of experimental properties in cuprates such as the oxidation energy, local moments, band gaps, and even stripe orders [13, 14, 27]. Increasing $U$ from 2 to 4eV results in a slightly larger copper local moment of about 0.53$\mu_B$, which is in better agreement with the experiments [25]. Increasing $U$ values in Fig.S 5(g-j) can also further raise the empty Cu bands to higher energy. In particular, the $U$ =4eV case shows an AFM gap between Cu bands of 1eV, which matches with experiment [28]. In addition, changing $U$ values can only make very little difference to the indirect band gap at the Fermi level by a very small amount. This is because the indirect band gap at the Fermi level is between the copper band at M' point and the bismuth band at X' point, which is unrelated to the empty Cu bands at high energy.

We have also performed similar calculations by changing the PBE+$U$ functional to the SCAN+$U$ functional. For transitional metal oxides, the plain SCAN method provides good predictions of the local moments but generally underestimates the band gaps [18]. In particular, it provides a metallic ground state in a wide range of insulators including oxides with Ti, V, Co, Ni, and Cu [19]. The improved SCAN+$U$ method can better reproduce the experimental band gaps and local moments, the optimal $U$ value for CuO is about 2eV for SCAN+$U$ method [19].

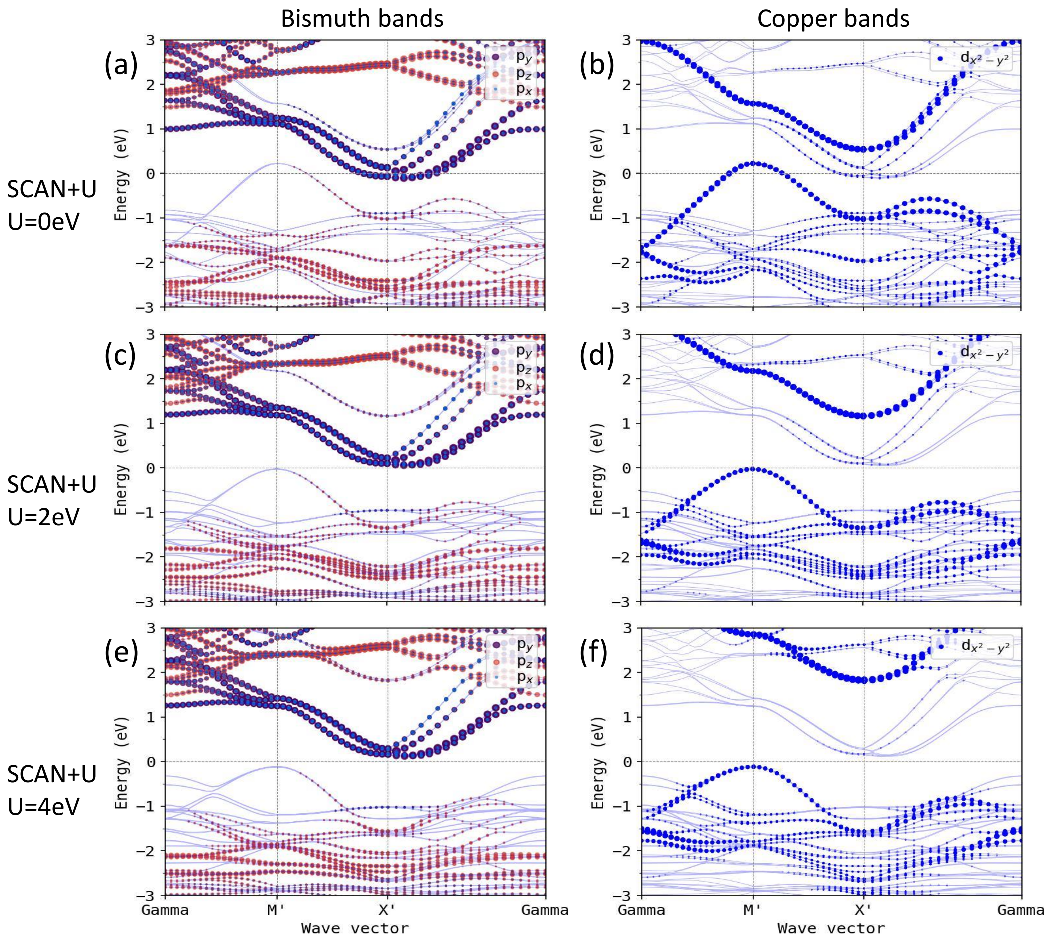


Fig.S 6: Projected band structures on the Bi $p$-orbitals and Cu $d_{x^2-y^2}$ orbitals from SCAN+$U$, with different $U$ values. Panels (a-b), (c-d), and (e-f) are the results of SCAN+$U$ with $U$ =0, 2, and 4eV, respectively. Panels (a)(c)(e) show the projections on Bi $p$-orbitals while panels (b)(d)(f) show Cu $d_{x^2-y^2}$ orbitals.

Figure.S 6 shows the band structures using the SCAN+$U$ method in Bi-2212. The $U$ =0eV calculations in Fig.S 6(a) and (b) show an AFM order, with a local moment of 0.43$\mu_B$ agrees with the previous SCAN study on Bi-2212 [4]. The local moment is about the same as PBE+$U$ with $U = 2eV$ in previous discussions. However, the SCAN method shows a metallic ground state. This is because the SCAN functional underestimates the AFM gap of Cu bands to about 0.3eV as shown in Fig.S 6(b), much smaller than the 1.0eV gap observed in experiment [28]. In addition, we find that SCAN+$U$ with $U$ = 2eV in Fig.S 6(c) and (d) can improve the band gap prediction just like in CuO. The local moment of the AFM order is 0.59$\mu_B$, slightly larger than the one given by PBE+$U$ with $U$ = 4eV.

As a conclusion, we find that for both PBE functional in Fig.S 5 and SCAN functional in Fig.S 6, the DFT+$U$ corrections with finite $U$ are always needed to have an insulating ground state. In PBE+$U$ calculation, $U$ =0eV happens to be non-magnetic, without any AFM gap opening for the Cu bands, so both electron and hole pockets at the Fermi level come from the Cu bands as shown in Fig.S 5(b). However, in SCAN+$U$ calculation, the $U$ =0eV case shows an AFM order, where the upper Cu bands show higher energy than the Bi bands at X' point due to the opening of an AFM gap. As a result, while the hole pockets at the Fermi level still come from the Cu bands at M' point, the electron pockets are now coming from the Bi bands at X' point as shown in Fig.S 6(b). For finite $U$ larger than 2eV, the choices of different functional and the values of $U$ affect the unoccupied bands, but make little difference on the occupied bands. Therefore, the DFT functional and values of $U$ will have negligible effects on our main results around or below the Fermi level, including the results of hole-doped systems as we will demonstrate in Sec. IV B. In our main article, we choose to use PBE+$U$ with $U$ = 4eV just to match the AFM gap size with experimental observation [28].

### B. Hole doped system

In this subsection, we focus on the most energetically favorable crystal structure of the hole-doped system and will show that the functional choice does not affect our results in the hole-doped system.

In prior benchmark studies, PBE+$U$ with $U$ = 4eV [13] and SCAN+$U$ with $U$ = 2eV [19] are known to reproduce the experimental band gaps and local magnetic moments in cuprates well. These two methods also provide similar results in undoped Bi-2212 as we discussed above. Here, in Fig.S 7 we study the 25% hole overdoped system and compare the unfolded band structures of the non-magnetic states from these two methods. There are some tiny differences between the two results, such as the SCAN+$U$ functional in Fig.S 7(b) shows slightly different projection weight compared to PBE+$U$ in Fig.S 7(a) on the $d_{xz/yz}$ and $d_{xy/z^2}$ orbitals between -3eV and -1eV. However, the main physics in BSCCO is on the $d_{x^2-y^2}$ orbitals and the bands near the Fermi level are almost the same from the two approaches. Hence, we conclude that the choice of functionals has little effect on our main results in the hole-doped system.

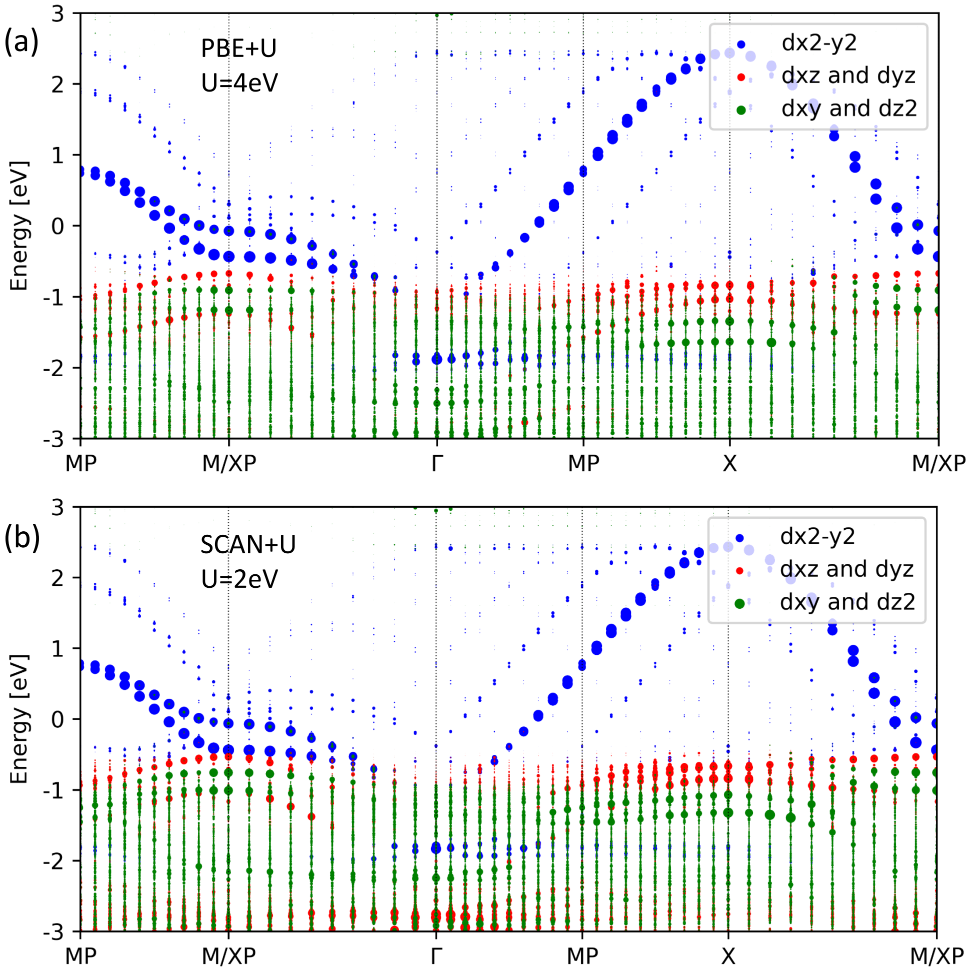


Fig.S 7: Unfolded band structures of the non-magnetic states from (a) PBE+$U$ with $U$ = 4eV and (b) SCAN+$U$ with $U$ = 2eV. The size of blue, red, and green dots represent the spectral weights of the $d_{x^2-y^2}$, $d_{xz/yz}$, and $d_{xy/z^2}$ orbitals of the Cu atoms.

## V. WANNIERIZATION

Wannierization is a widely used post-processing technique in DFT calculation that enables the transformation of electronic wavefunctions obtained from plane-wave basis sets into a set of localized real-space functions called Wannier functions [29]. By constructing the maximally-localized Wannier functions [30], one can then extract tight-binding models from the DFT calculations using the Wannier basis, which offer a more intuitive and physically meaningful interpretation of the electronic properties of materials and are a powerful tool for investigating their electronic structure [31]. The software that we used for the Wannierization is the Wannier90 v3.0 package [32].

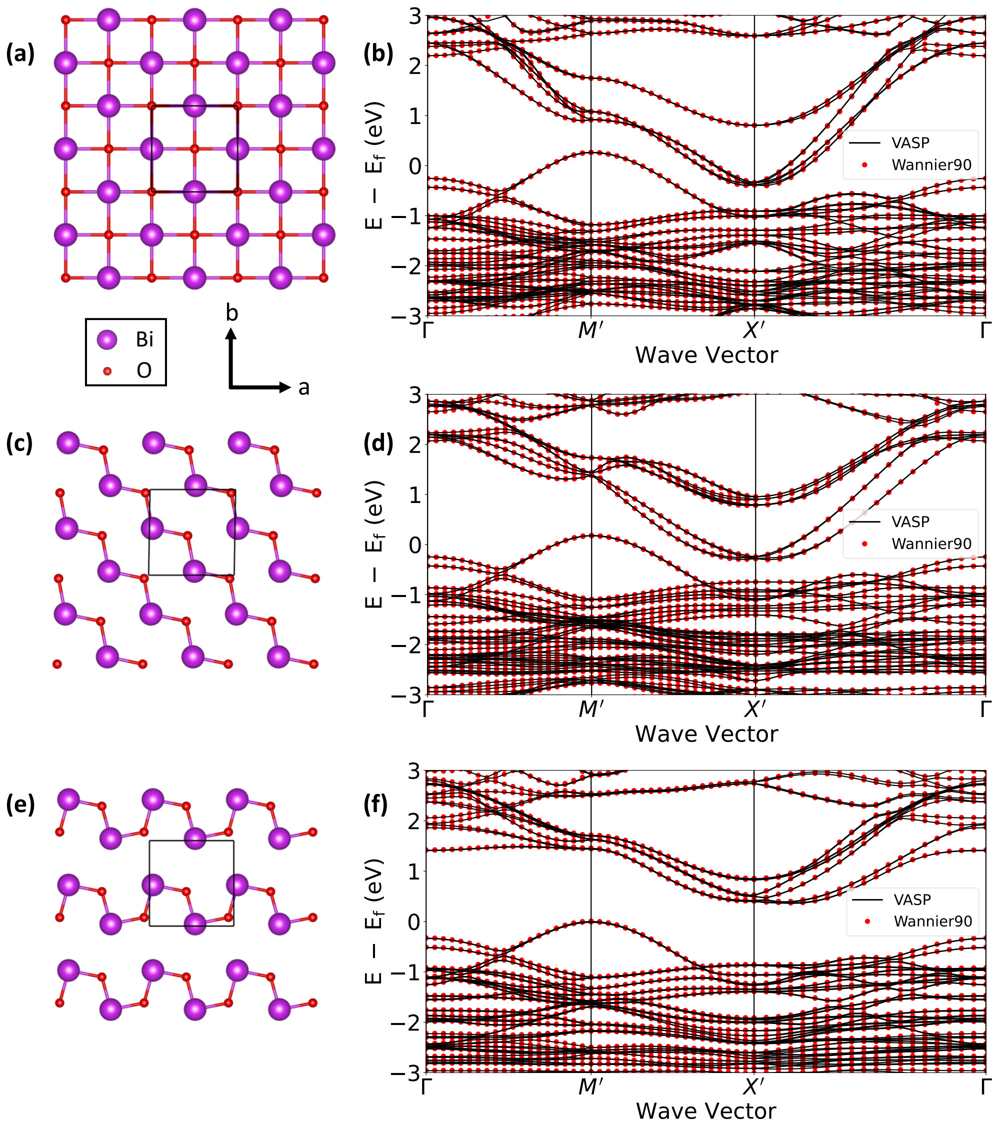


Fig.S 8: Wannierization in the undoped system. (a) Top view of the high-symmetry crystal structure. (b) The band structures of the high-symmetry crystal structure. The black solid lines are the band structure directly computed by VASP, while the red dots are the band structure from the extracted tight-binding Hamiltonian on the Wannier basis. (c) and (e) Top views of two low-symmetry crystal structures. (d) and (f) The corresponding band structures from crystals in (c) and (e).

Due to the heavy computational cost, the Wannierization is usually performed in a subspace of the whole Hilbert space. The choice of such subspace depends on the orbitals that are of interest. In the undoped system, besides the Cu atoms, the Bi atoms also play a crucial role around the Fermi level, as shown in Fig.S 5 and 6 and in many previous studies [4, 6, 22, 33]. In addition, we also want to study the impact of Bi-O coupling strength on the band gaps. Based on the

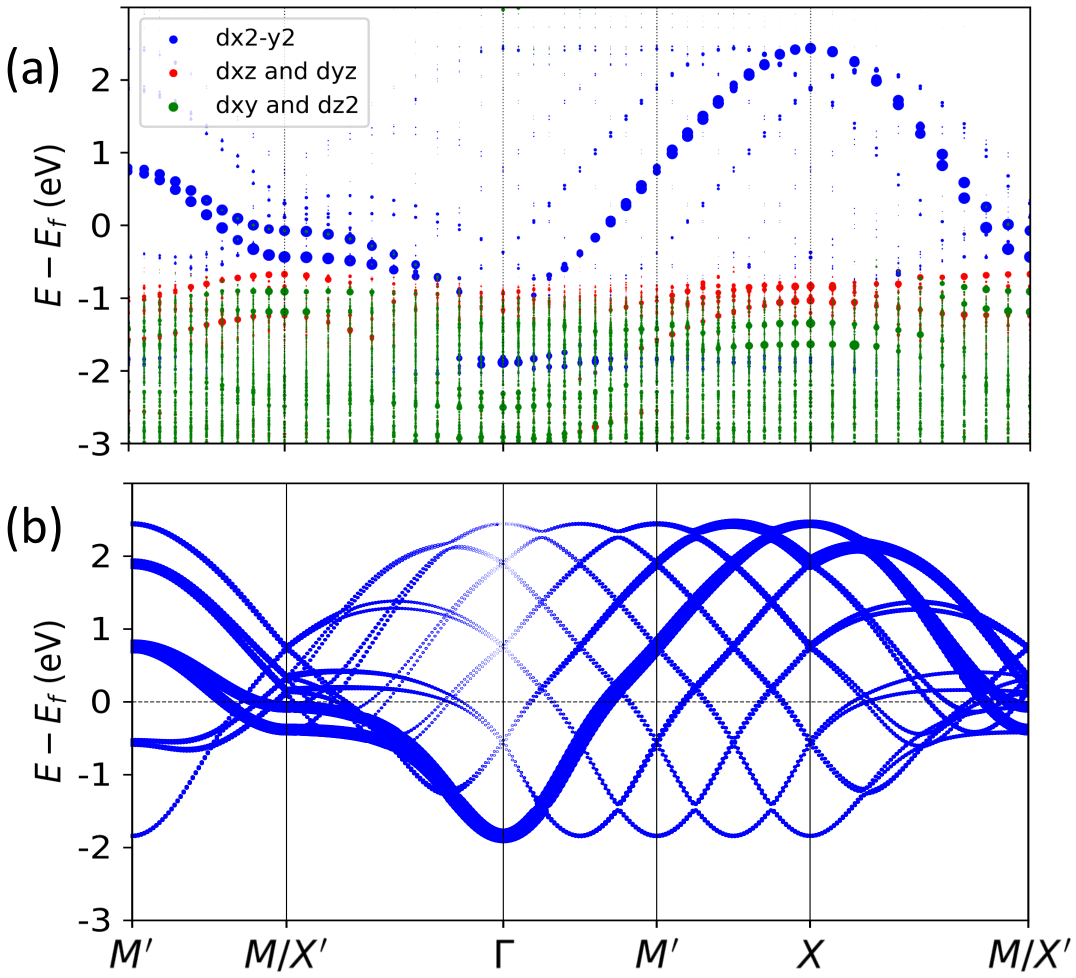


Fig.S 9: Wannierization in the 25% hole-doped system (non-magnetic state). (a) Unfolded band structure directly computed by VASP. The blue, red, and green dots represent the $d_{x^2-y^2}$, $d_{xz} + d_{yz}$, and $d_{xy} + d_{z^2}$ orbitals of the copper atoms, respectively. The sizes of the dots represent the weight of the orbitals on each band. (b) The unfolded band structure of the Cu-$d_{x^2-y^2}$ Wannier orbitals from the Wannierized tight-binding model.

above considerations, we perform Wannierization on the subspace spanned by Cu-$d$, Bi-$p$, and O-$p$ orbitals, resulting in a 160-band tight-binding model. Figure.S 8 shows the crystals and compares the corresponding band structures from VASP and the Wannierized tight-binding models. The band structures from the two methods are in perfect agreement with each other. This is because the selected Wannier orbitals hardly couple to the semi-core or high-energy conducting bands in this system such as the orbitals from O-$s$, Bi-$s$, Sr, and Ca. Hence, the Hilbert subspace spanned by the Cu-$d$, Bi-$p$, and O-$p$ orbitals provides a great description of the bands around the Fermi level.

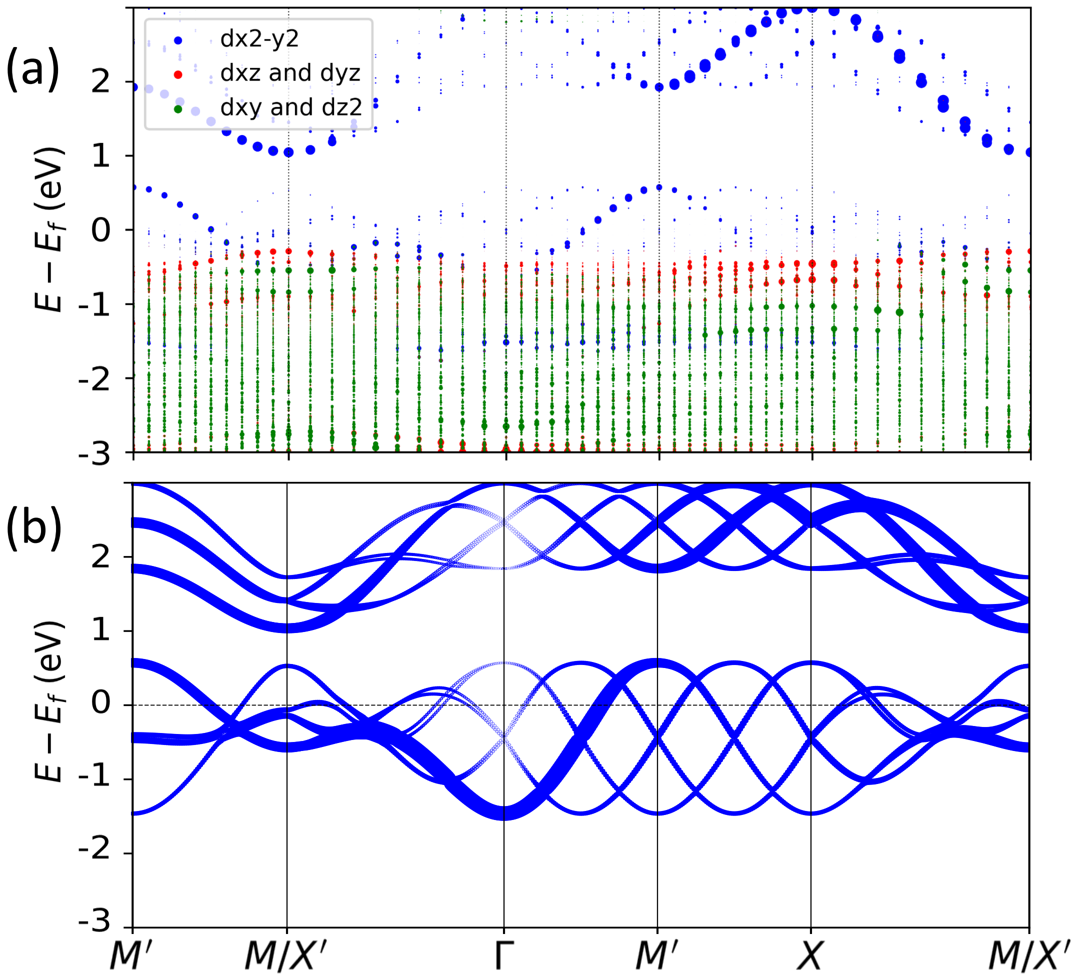


Fig.S 10: Wannierization in the 25% hole-doped system (GAFM state). (a) Unfolded band structure directly computed by VASP. The blue, red, and green dots represent the $d_{x^2-y^2}$, $d_{xz}+d_{yz}$, and $d_{xy}+d_{z^2}$ orbitals of the copper atoms, respectively. The sizes of the dots represent the weight of the orbitals on each band. (b) The unfolded band structure of the Cu-$d_{x^2-y^2}$ Wannier orbitals from the Wannierized tight-binding model.

The 25% hole-doped crystal has a much larger 244-atom unit cell as shown in Fig.S 4(a) above. To reduce the computational cost, we only capture the dominant physics by focusing on the bands crossing the Fermi level. We notice that the Bi bands are raised to high energy away from the Fermi level due to the hole doping, which is consistent with several previous studies [5, 22]. In addition, most of the Cu $d$-shell orbitals are fully occupied below the Fermi level except for the $d_{x^2-y^2}$ orbitals as shown in Fig.S 9(a), 10(a), and 11(a). Hence, a subspace with only Cu-$d_{x^2-y^2}$ Wannier orbitals should be able to capture the dominant physics in this system.

Figure.S 9(a) and (b) show the unfolded band structures of the non-magnetic states from VASP

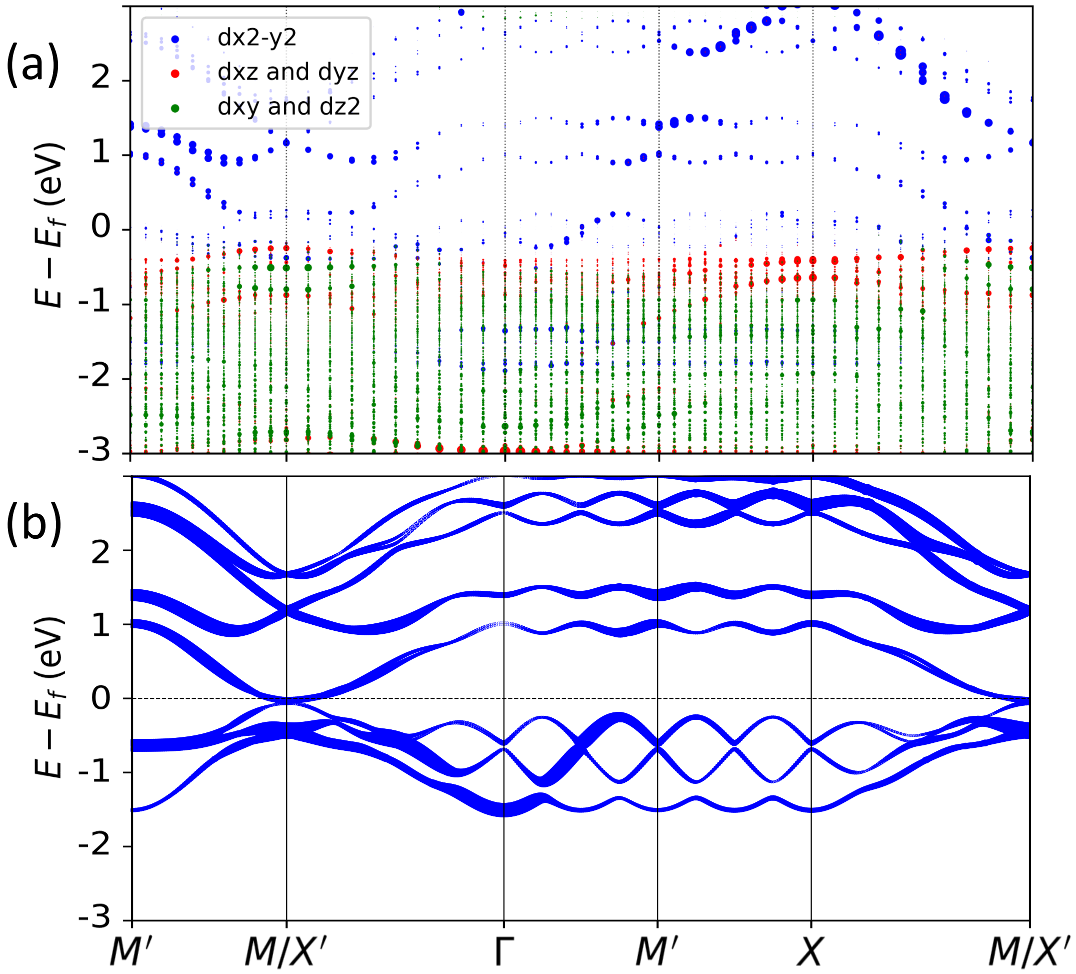


Fig.S 11: Wannierization in the 25% hole-doped system (stripe-order state). (a) Unfolded band structure directly computed by VASP. The blue, red, and green dots represent the $d_{x^2-y^2}$, $d_{xz} + d_{yz}$, and $d_{xy} + d_{z^2}$ orbitals of the copper atoms, respectively. The sizes of the dots represent the weight of the orbitals on each band. (b) The unfolded band structure of the Cu-$d_{x^2-y^2}$ Wannier orbitals from the Wannierized tight-binding model.

and the Wannierized tight-binding models. The Wannierized models successfully capture the main $d_{x^2-y^2}$ bands of the unfolded band structure from VASP. Around the Fermi level, there are two branches of flat bands around the antinodal region (the $M/X'$ point in the figure). They are split by interlayer coupling in the bilayers, consistent with the ARPES experiments [34, 35]. In contrast, the nodal region locates between Γ and $M'$, consistent with experiments [36], where the bands are not flattened. Going along $\Gamma \to M' \to X$, one can see four bands crossing the Fermi level with increasing energy along the $k$-point path and four bands crossing the Fermi level with decreasing energy. These bands are crucial to the shadow bands in the Fermi surface as discussed in the main

article.

Figure.S 10 and 11 show the unfolded band structures of GAFM and stripe-order states from VASP and the corresponding Wannierized tight-binding models. The band structures from Wannierized models successfully capture the main $d_{x^2-y^2}$ bands of the unfolded band structure from VASP.

## VI. UNIFORM MAGNETIC STATES AND THEIR ENERGIES IN HOLE-DOPED SYSTEM

In this section, we study the magnetic orders with almost uniform local moments in the hole-doped system. We initialize the local moments of the Cu atoms in different magnetic orders and converge both electronic and crystal structures. The most energetically favorable magnetic order among them is the G-AFM order, where for each copper atom, the nearest-neighbor copper atoms in the $ab$ plane or along the $\pm z$ direction are aligned antiparallel to it as illustrated in Fig.S 12(a).

In addition to the G-AFM state, we also find several meta-stable magnetic orders. Fig.S 12(b) shows the C-AFM state, where the interlayer Cu spins in one bilayer are aligned parallel. Fig.S 12(c) shows the A-AFM state, where the intralayer Cu spins are aligned parallel. The intralayer parallel-aligned spins cost much more energy than the interlayer ones because the intralayer hopping scales one order of magnitude larger than the interlayer hoppings, according to the Wannierized tight-binding model in Supp. Sec. V. Fig.S 12(d) shows the FM state, where all the Cu spins are aligned parallel. We have also stabilized the C′-AFM state, whose spin structure is the same as the G-AFM state, except for the nearest-neighbor interbilayer spins are now aligned parallel. Due to the small interbilayer hoppings between Cu atoms (<0.001 meV according to Wannierization results), the energy difference between C′-AFM and G-AFM is negligible. For the same reason, we will only focus on one bilayer of the system in the following discussion.

## VII. DFT ORBITALS VS WANNIER ORBITALS

In this section, we will compare the VASP atomic projection and the Wannier orbital projection. We will show the problems of using the VASP atomic projections to understand the stripe ordering states. Figure. S13 shows the local moments and occupancies projected on the VASP Cu $d$-shell orbitals. They both show a similar wavy pattern to the Wannier orbitals results in the main article, but the modulations are much weaker in amplitude: in particular, the modulations of the total

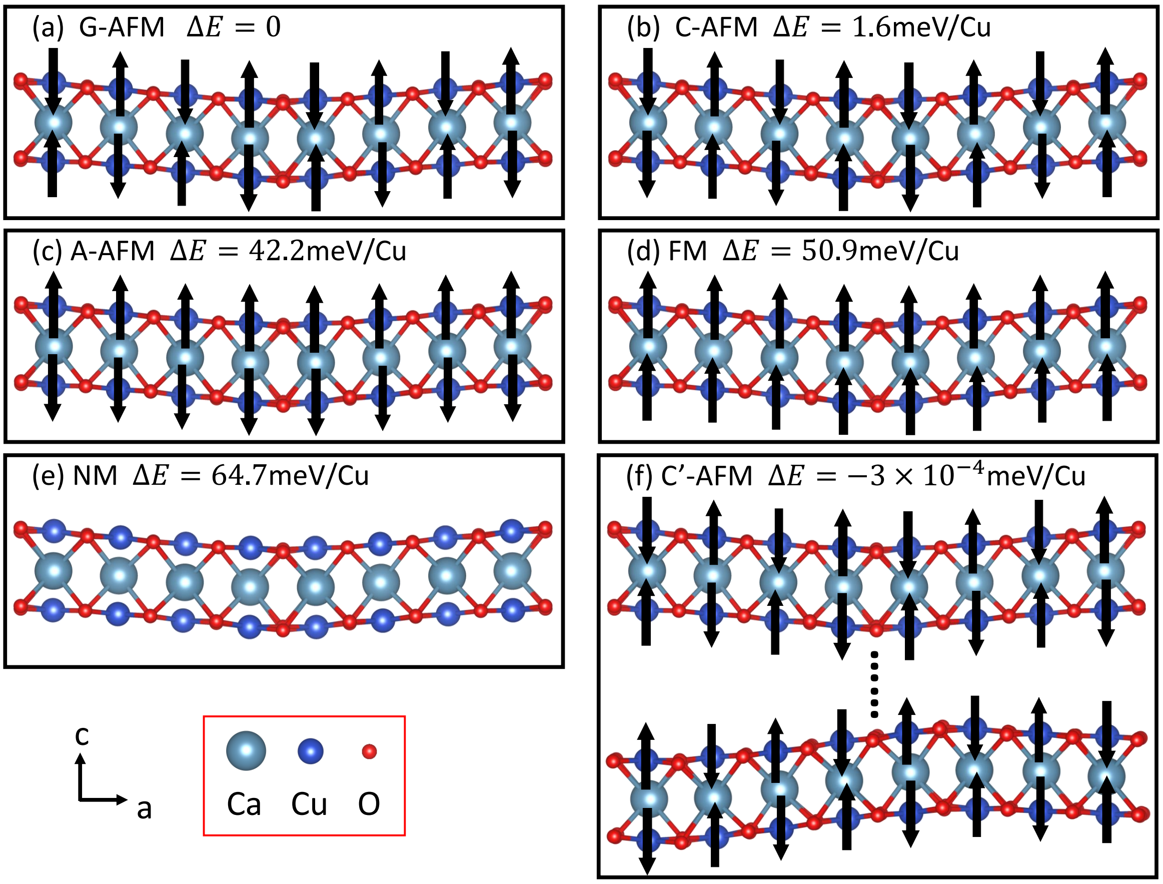


Fig.S 12: Six different spin structures in the hole-doped system and their energies. Each unit cell contains two bilayers as shown in Fig.S 4(a). However, for the spin structures in (a-e), we only illustrate one of the bilayers for simplicity, while the other bilayer has the same spin structure. (a) The G-AFM state, whose energy is set as the reference energy $\Delta E \equiv E - E_{\mathrm{GAFM}}$. The black arrows represent the spin directions of the Cu atoms. (b) The C-AFM state, where the two layers are FM coupled to each other instead of the AFM coupling in the G-AFM case. (c) The A-AFM state, where the in-plane nearest-neighbor Cu atoms are FM coupled to each other. (d) The FM state, where both intra- and inter-layer nearest-neighbor Cu atoms are FM coupled to each other. (e) The non-magnetic state, where all local moments are zero. (f) The C′-AFM state, where the intra-bilayer spin structure is the same as the one in G-AFM, while all the spins in the other bilayer are flipped compared to G-AFM. The two bilayers are FM coupled to each other instead of the AFM coupling in the G-AFM case.

occupancy $n_d$ are one order of magnitude smaller than those of the magnetic moment which is very hard to understand physically. Part of the problem is due to the incompleteness of the VASP projection basis and its lack of orthonormality. For example, by integrating the projected density of states on Cu-site $d$-shell and O-site $p$-shell atomic orbitals, we find about 0.036 holes/$CuO_2$ doped

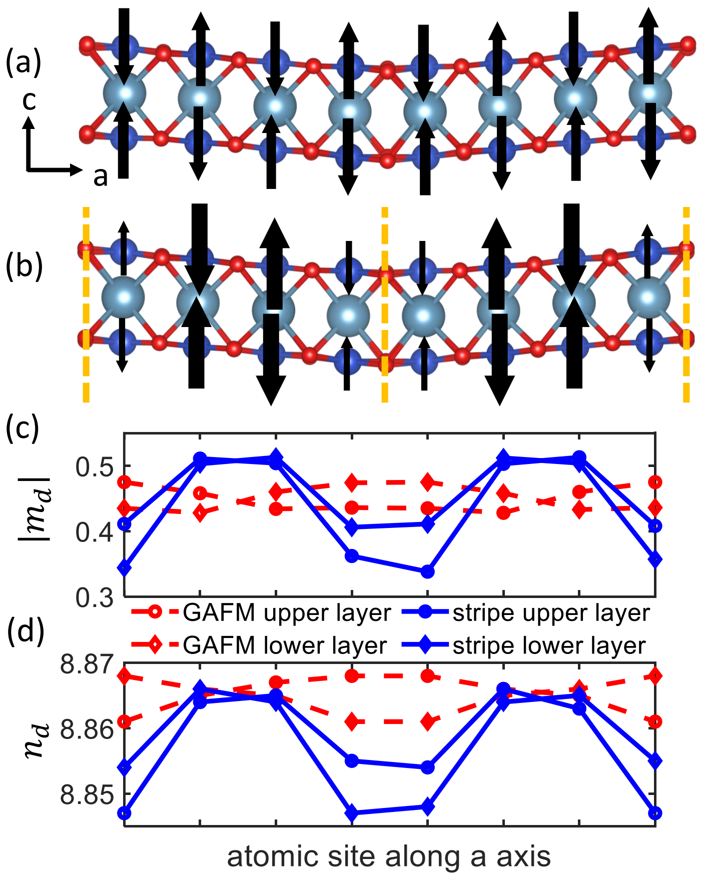


Fig.S 13: VASP projected Cu sites' $d$-shell local moments and occupancies. (a) and (b) Illustrations of G-AFM and the stripe order phase adapted from Fig. 5 of the main text. (c) The amplitude of local moments ($\mu_B$) on Cu atomic sites along $a$-axis from VASP. (d) The $d$-shell occupancy on Cu atomic sites given by VASP. Red dashed lines and blue solid lines represent the G-AFM and stripe-order states, respectively. Circles and diamonds show the results of the upper and lower layers.

into the Cu $d$-shell orbitals and about 0.16 holes/$CuO_2$ holes doped into the O $p$-shell orbitals. The oxygen hole content is very large and makes the interpretation of the Cu moments and occupancies incomplete. In addition, these hole-dopings do not sum up to the correct hole-doping level (0.25) because the projections produced by VASP are not orthonormal.

# VIII. SUMMARY OF COMPUTATIONAL DETAILS

## A. SIESTA

The SIESTA package is only used to approximately relax the hole-doped crystal (244-atom unit cell) in order to create a chemically reasonable starting point for further crystal relaxation in VASP. PBE pseudo-potentials are obtained from ABINIT's pseudo database [37, 38]. We use the PBE+$U$ functional with $U = 4$ eV added only to the Cu $d$-orbitals. DZP basis with EnergyShift of 100 meV and SplitNorm of 0.25 is used in all SIESTA calculations. The $k$ grid is chosen as $2 \times 7 \times 1$, with a high mesh cutoff energy of 600 Ry. The maximum $l$-quantum number is 3 for Sr and 2 for all other elements. All SIESTA calculations converge to an energy tolerance of $10^{-4}$ eV and a force tolerance of 0.05 eV/Å.

## B. VASP

The 5.4.4 version of the VASP package and the PAW pseudo potentials of PBE version 54 are used for all calculations. All DFT+$U$ calculations add $U$ corrections only to the Cu $d$-orbitals using the simplified (rotationally invariant) approach (LDAUTYPE = 2) [39], with maximum $l$-quantum number set to 4. All VASP calculations converge to an energy tolerance of $10^{-5}$ eV and a force tolerance of 0.03 eV/Å. The convergence of plane-wave cutoff energy, $k$-mesh, and Gaussian smearing are demonstrated in the convergence tests above.


[1] G. Kresse and J. Furthmüller, Computational materials science **6**, 15 (1996), URL https://www.sciencedirect.com/science/article/abs/pii/0927025696000080.

[2] G. Kresse and J. Furthmüller, Phys. Rev. B **54**, 11169 (1996), URL https://link.aps.org/doi/10.1103/PhysRevB.54.11169.

[3] C. Yelpo, R. Faccio, D. Ariosa, and S. Favre, Journal of Physics: Condensed Matter **33**, 185705 (2021), URL https://iopscience.iop.org/article/10.1088/1361-648X/abed17.

[4] J. Nokelainen, C. Lane, R. S. Markiewicz, B. Barbiellini, A. Pulkkinen, B. Singh, J. Sun, K. Pussi, and A. Bansil, Phys. Rev. B **101**, 214523 (2020), URL https://link.aps.org/doi/10.1103/PhysRevB.101.214523.

[5] Y. He, T. S. Nunner, P. J. Hirschfeld, and H.-P. Cheng, Phys. Rev. Lett. **96**, 197002 (2006), URL https://link.aps.org/doi/10.1103/PhysRevLett.96.197002.

[6] K. Foyevtsova, H. C. Kandpal, H. O. Jeschke, S. Graser, H.-P. Cheng, R. Valentí, and P. J. Hirschfeld, Phys. Rev. B **82**, 054514 (2010), URL https://link.aps.org/doi/10.1103/PhysRevB.82.054514.

[7] W. Fan and Z. Zeng, Superconductor Science and Technology **24**, 105007 (2011), URL https://iopscience.iop.org/article/10.1088/0953-2048/24/10/105007.

[8] A. J. Cohen, P. Mori-Sánchez, and W. Yang, Science **321**, 792 (2008).

[9] J. P. Perdew and M. Levy, Phys. Rev. Lett. **51**, 1884 (1983), URL https://link.aps.org/doi/10.1103/PhysRevLett.51.1884.

[10] J. P. Perdew and A. Zunger, Phys. Rev. B **23**, 5048 (1981), URL https://link.aps.org/doi/10.1103/PhysRevB.23.5048.

[11] V. I. Anisimov, J. Zaanen, and O. K. Andersen, Phys. Rev. B **44**, 943 (1991), URL https://link.aps.org/doi/10.1103/PhysRevB.44.943.

[12] N. E. Kirchner-Hall, W. Zhao, Y. Xiong, I. Timrov, and I. Dabo, Applied Sciences **11**, 2395 (2021).

[13] L. Wang, T. Maxisch, and G. Ceder, Phys. Rev. B **73**, 195107 (2006), URL https://link.aps.org/doi/10.1103/PhysRevB.73.195107.

[14] L. Deng, Y. Zheng, Z. Wu, S. Huyan, H.-C. Wu, Y. Nie, K. Cho, and C.-W. Chu, Proceedings of the National Academy of Sciences **116**, 2004 (2019), URL https://www.pnas.org/doi/abs/10.1073/pnas.1819512116.

[15] J. Sun, A. Ruzsinszky, and J. P. Perdew, Phys. Rev. Lett. **115**, 036402 (2015), URL https://link.aps.org/doi/10.1103/PhysRevLett.115.036402.

[16] M. Ekholm, D. Gambino, H. J. M. Jönsson, F. Tasnádi, B. Alling, and I. A. Abrikosov, Phys. Rev. B **98**, 094413 (2018), URL https://link.aps.org/doi/10.1103/PhysRevB.98.094413.

[17] F. Tran, G. Baudesson, J. Carrete, G. K. H. Madsen, P. Blaha, K. Schwarz, and D. J. Singh, Phys. Rev. B **102**, 024407 (2020), URL https://link.aps.org/doi/10.1103/PhysRevB.102.024407.

[18] G. Sai Gautam and E. A. Carter, Phys. Rev. Mater. **2**, 095401 (2018), URL https://link.aps.org/doi/10.1103/PhysRevMaterials.2.095401.

[19] O. Y. Long, G. Sai Gautam, and E. A. Carter, Phys. Rev. Mater. **4**, 045401 (2020), URL https://link.aps.org/doi/10.1103/PhysRevMaterials.4.045401.

[20] L. F. Mattheiss and D. R. Hamann, Phys. Rev. B **38**, 5012 (1988), URL https://link.aps.org/doi/10.1103/PhysRevB.38.5012.

[21] M. S. Hybertsen and L. F. Mattheiss, Phys. Rev. Lett. **60**, 1661 (1988), URL https://link.aps.org/doi/10.1103/PhysRevLett.60.1661.

[22] H. Lin, S. Sahrakorpi, R. S. Markiewicz, and A. Bansil, Phys. Rev. Lett. **96**, 097001 (2006), URL https://link.aps.org/doi/10.1103/PhysRevLett.96.097001.

[23] D. Song, X. Zhang, C. Lian, H. Liu, I. Alexandrou, I. Lazić, E. G. Bosch, D. Zhang, L. Wang, R. Yu, et al., Advanced Functional Materials **29**, 1903843 (2019), URL https://onlinelibrary.wiley.com/doi/10.1002/adfm.201903843.

[24] Y. He, S. Graser, P. J. Hirschfeld, and H.-P. Cheng, Phys. Rev. B **77**, 220507 (2008), URL https:

//link.aps.org/doi/10.1103/PhysRevB.77.220507.

[25] J. R. Schrieffer and J. S. Brooks, Handbook of high-temperature superconductivity: theory and experiment (Springer New York, NY, 2007), 1st ed.

[26] C. Lane, J. W. Furness, I. G. Buda, Y. Zhang, R. S. Markiewicz, B. Barbiellini, J. Sun, and A. Bansil, Phys. Rev. B **98**, 125140 (2018), URL https://link.aps.org/doi/10.1103/PhysRevB.98.125140.

[27] S. Pesant and M. Côté, Phys. Rev. B **84**, 085104 (2011), URL https://link.aps.org/doi/10.1103/PhysRevB.84.085104.

[28] Z. Wang, C. Zou, C. Lin, X. Luo, H. Yan, C. Yin, Y. Xu, X. Zhou, Y. Wang, and J. Zhu, Science **381**, 227 (2023), URL https://www.science.org/doi/10.1126/science.add3672.

[29] G. H. Wannier, Phys. Rev. **52**, 191 (1937), URL https://link.aps.org/doi/10.1103/PhysRev.52.191.

[30] N. Marzari and D. Vanderbilt, Phys. Rev. B **56**, 12847 (1997), URL https://link.aps.org/doi/10.1103/PhysRevB.56.12847.

[31] N. Marzari, A. A. Mostofi, J. R. Yates, I. Souza, and D. Vanderbilt, Rev. Mod. Phys. **84**, 1419 (2012), URL https://link.aps.org/doi/10.1103/RevModPhys.84.1419.

[32] G. Pizzi, V. Vitale, R. Arita, S. Blügel, F. Freimuth, G. Géranton, M. Gibertini, D. Gresch, C. Johnson, T. Koretsune, et al., Journal of Physics: Condensed Matter **32**, 165902 (2020), URL https://iopscience.iop.org/article/10.1088/1361-648X/ab51ff/meta.

[33] L.-L. Wang, P. J. Hirschfeld, and H.-P. Cheng, Phys. Rev. B **72**, 224516 (2005), URL https://link.aps.org/doi/10.1103/PhysRevB.72.224516.

[34] Y. He, S.-D. Chen, Z.-X. Li, D. Zhao, D. Song, Y. Yoshida, H. Eisaki, T. Wu, X.-H. Chen, D.-H. Lu, et al., Phys. Rev. X **11**, 031068 (2021), URL https://link.aps.org/doi/10.1103/PhysRevX.11.031068.

[35] Y. He, M. Hashimoto, D. Song, S.-D. Chen, J. He, I. Vishik, B. Moritz, D.-H. Lee, N. Nagaosa, J. Zaanen, et al., Science **362**, 62 (2018), URL https://www.science.org/doi/10.1126/science.aar3394.

[36] J. A. Sobota, Y. He, and Z.-X. Shen, Rev. Mod. Phys. **93**, 025006 (2021), URL https://link.aps.org/doi/10.1103/RevModPhys.93.025006.

[37] X. Gonze, J.-M. Beuken, R. Caracas, F. Detraux, M. Fuchs, G.-M. Rignanese, L. Sindic, M. Verstraete, G. Zerah, F. Jollet, et al., Computational Materials Science **25**, 478 (2002).

[38] X. Gonze, B. Amadon, P.-M. Anglade, J.-M. Beuken, F. Bottin, P. Boulanger, F. Bruneval, D. Caliste, R. Caracas, M. Côté, et al., Computer Physics Communications **180**, 2582 (2009).

[39] S. L. Dudarev, G. A. Botton, S. Y. Savrasov, C. J. Humphreys, and A. P. Sutton, Phys. Rev. B **57**, 1505 (1998), URL https://link.aps.org/doi/10.1103/PhysRevB.57.1505.
